# Supplementary material for: Enhancing Offline Model-Based RL via Active Model Selection: A Bayesian Optimization Perspective
Source: arXiv:2502.11480 source file (2026-10-18)
Supplement: Supplementary file 1 [file appendix-dummy.tex]

\newpage
\citep{janner2019trust, lu2021revisiting, argenson2020model, matsushima2020deployment},
\citep{yu2020mopo},
\citep{kidambi2020morel},
\citep{rigter2022rambo},
\citep{yu2021combo},
\citep{bhardwaj2023adversarial}
\citep{fujimoto2019off, wu2019behavior, kumar2019stabilizing, nair2020awac, fujimoto2021minimalist, wang2022diffusion},
\citep{kumar2020conservative, kostrikov2021offline, bai2022pessimistic},
\citep{an2021uncertainty, wu2021uncertainty, bai2022pessimistic}
\citep{vemula2023virtues}
